# Supplementary material for: Benchmarking noisy label detection methods
Source: arXiv:2510.16211 source file (2026-08-21)
Supplement: Supplementary file 1 [file learnability.tex]

Assuming that our set of samples $\dataset$ comes from a joint probability distribution $\probabilityop(\samplefeature, \samplelabel)$ determined by the generative model $\probabilityop(\samplefeature|\samplelabel)$ and a prior probability distribution $\probabilityop(\samplelabel)$, we can obtain the posterior probability of a class given a sample by the definition of conditional probability and the Bayes' theorem
\begin{equation}
    \probabilityop(\samplelabel|\samplefeature) = \frac{\probabilityop(\samplefeature, \samplelabel)}{\probabilityop(\samplefeature)} = \frac{\probabilityop(\samplefeature|\samplelabel)\probabilityop(\samplelabel)}{\sum_{\samplelabel'} \probabilityop(\samplefeature|\samplelabel')\probabilityop(\samplelabel')},
\end{equation}
where $\samplelabel \in [1, \dots, \numberofclasses]$ indicates the class and $\samplefeature \in \featurespace$ indicates the sample features. In a label noise scenario, we observe instead the noisy posterior $P(\tilde{y}|X)$. 
The relation between $\samplelabelnoisy$ and $\samplelabel$ is given by the noise transition function $\probabilityop(\samplelabelnoisy|\samplelabel, \samplefeature)$. Thus, we can write the noisy posterior
\begin{equation}
    P(\tilde{y}|X) = \sum_y P(\tilde{y}|y, X)P(y|X).
    \label{eq:noisy_posterior}
\end{equation}
With this, we define that a sample $x$ is impossible to learn when the Bayes' classifier of the noisy posterior and the Bayes' classifier of the clean posterior have different predictions, that is
\begin{equation}
    \argmax_{k \in [1, \dots \numberofclasses]} P(\tilde{y}|X=x) \neq \argmax_{k \in [1, \dots \numberofclasses]} P(y|X=x)
    \label{eq:bayes_learnability}
\end{equation}
in the sense that the model will at best learn the noisy posterior, which will disagree with the clean posterior. This means that, without any further constraints on the problem, there is no hope of learning the correct class of this sample. This definition also separates the effect of ambiguity, which is captured by the clean posterior, and label noise, captured by the transition function.

We can analyze what this learnability definition means for the noise models we defined before. For example, in the symmetric noise model, take a sample $x$ with clean posterior $p_i = P(y =i|X=x)$ that is maximized by $i=k$. We need that the noisy posterior, from Equation \ref{eq:noisy_posterior} and Equation \ref{eq:symmetric_noise}, given by
\begin{align}
    \tilde{p}_i &= P(\tilde{y}=i|X=x) \\
    &= (1-\eta)p_i + \frac{\eta}{\numberofclasses-1} \sum_{j \in [1, \dots, \numberofclasses] \backslash i} p_j \\
    &= (1-\eta)p_i + \frac{\eta}{\numberofclasses-1} (1 - p_i) \\
    &= \frac{\eta}{\numberofclasses-1} + \left(1-\eta - \frac{\eta}{\numberofclasses-1} \right) p_i
\end{align}
be maximized for $k$ as well. Thus, for a sample to be learnable, we need that, for all $i \neq k$,
\begin{align}
\tilde{p}_k &> \tilde{p}_i \\
\frac{\eta}{\numberofclasses-1} + \left(1-\eta - \frac{\eta}{\numberofclasses-1} \right) p_k &> \frac{\eta}{\numberofclasses-1} + \left(1-\eta - \frac{\eta}{\numberofclasses-1} \right) p_i \\
\
\left(1-\eta - \frac{\eta}{\numberofclasses-1} \right) (p_k - p_i) &> 0 \\
\
\left(1-\eta - \frac{\eta}{\numberofclasses-1} \right) &> 0 \\
\
\eta\left(1 + \frac{1}{\numberofclasses-1}\right) &< 1 \\
\eta &< \frac{1}{1 + \frac{1}{\numberofclasses-1}} \\
\eta &< \frac{\numberofclasses-1}{\numberofclasses}.
\end{align}
% \begin{align}
%     \tilde{p}_k &> \tilde{p}_i \\
%     (1-\eta)p_k + \frac{\eta}{\numberofclasses-1} \sum_{l \in [1, \dots, \numberofclasses] \backslash k} p_l &> (1-\eta)p_i + \frac{\eta}{\numberofclasses-1} \sum_{j \in [1, \dots, \numberofclasses] \backslash i} p_j \\
%     \
%     (1-\eta)p_k + \frac{\eta}{\numberofclasses-1} \left(p_i + \sum_{l \in [1, \dots, \numberofclasses] \backslash \{k, i\}} p_l\right) &> (1-\eta)p_i + \frac{\eta}{\numberofclasses-1} \left(p_k + \sum_{j \in [1, \dots, \numberofclasses] \backslash \{k, i\}} p_j\right) \\
%     \
%     (1-\eta)p_k + \frac{\eta}{\numberofclasses-1} p_i &> (1-\eta)p_i + \frac{\eta}{\numberofclasses-1} p_k \\
%     \eta(p_i - p_k + \frac{1}{\numberofclasses-1}(p_i - p_k)) &> p_i - p_k \\
%     \
%     \eta(p_i - p_k)(1 + \frac{1}{\numberofclasses-1}) &> p_i - p_k \\
%     \eta(1 + \frac{1}{\numberofclasses-1}) &< 1 \\
%     \eta &< \frac{1}{1 + \frac{1}{\numberofclasses-1}} \\
%     \eta &< \frac{\numberofclasses-1}{\numberofclasses}.
% \end{align}
Thus, $\eta^* = \frac{\numberofclasses-1}{\numberofclasses}$ is the tipping point of the problem, which is a known limit for symmetric noise \cite{oyen_robustness_2022}. If the noise rate goes over this value, the sample $x$ is unlearnable. In fact, the tipping point does not depend on $x$, meaning that if the noise rate is above this value, the problem is globally unlearnable (i.e, all the points in the sample space are unlearnable). 

%If the noise rate is known to be above the tipping point, it is possible to adjust the labels and make the problem learnable again. For example, for $\numberofclasses=2$ we have $\eta^* = 0.5$ if we assume noise rate above it $\eta = 0.7$, swapping the labels for both classes leaves us with $\eta = 0.3$. This is only possible, however, if the entire noise model is known. If it is known that the noise model is symmetric and the noise rate is above its tipping point, the correction can be performed. However, note that it is difficult to estimate the noise rate, even more difficult is to determine the noise model. In short, having these information constrains the problem further and allows for learning even when the problem is unlearnable.

If the noise rate is known to exceed the tipping point, it is sometimes possible to relabel the data and restore learnability. For instance, in the binary case ($\numberofclasses = 2$), the tipping point is $\eta^*=0.5$. If the actual noise rate is $\eta = 0.7$ and the noise model is symmetric, swapping the labels of both classes effectively reduces the noise rate to $\eta=0.3$, bringing it below the tipping point. However, this correction is only feasible if the noise model is fully known. In particular, knowing that the noise is symmetric and that the rate exceed the tipping point enables such adjustments. Still, estimating the true noise rate is challenging, and identifying the exact noise model is even more difficult. In summary, while this additional information can make an otherwise unlearnable problem solvable, it constitutes an external constraint on the problem and thus falls outside our original definition of learnability.

Now, for the pairwise noise model
\begin{equation}
    P(\tilde{y}=i|y=j, X) = \begin{cases}
        1-\eta & \text{if } i = j \\
        \eta & \text{if } i = j+1 \bmod \numberofclasses \\
        0 & \text{otherwise}
    \end{cases},
\end{equation}
the noisy posterior is given by
\begin{align}
    \tilde{p}_i &= P(\tilde{y}=i|X) \\
    &= (1-\eta)p_i + \eta p_{i-1 \bmod \numberofclasses}
\end{align}
and a sample $x$ with true class $k = \argmax_y P(y|X)$ is learnable when
\begin{align}
    \tilde{p}_k > \tilde{p}_{j} \quad \forall j \neq k.
\end{align}
Take $j = k+1 \bmod \numberofclasses$ and $l = k-1 \bmod \numberofclasses$, we have that: 
\begin{align}
    \tilde{p}_k &> \tilde{p}_{j} \\
    (1-\eta)p_k + \eta p_l &> (1-\eta)p_j + \eta p_k \\
    \eta(2p_k - p_j - p_l) &< p_k - p_j\\
    \eta &< \frac{p_k - p_j}{2p_k - p_j - p_l}
\end{align}
Now the learnability of the sample also depends on the clean posterior (and thus, on $x$), making it difficult to make a statement about the global learnability of the problem. We can however notice a few important aspects such as the fact that label noise is more impactful near the decision boundary. Intuitively this makes sense because for these samples the model is less certain and so it is easier to be swayed by the noise. Assuming the clean posterior is a continuous function, one of the decision boundaries will be on regions where $p_j \approx p_k \neq p_l$, in this case the learnability condition becomes $\eta \approx 0$. This matches with our intuition since it means that in these regions any amount of noise will make the model learn the wrong class.

The converse is also true, when $p_j = 0$ the learnability condition becomes $\eta < \frac{p_k}{2p_k - p_l}$ which can be as high as $1$ when $p_l \approx p_k$ meaning the sample is learnable for any noise rate. This also makes intuitive sense, for example, suppose that the sample is being confused between cats and dogs, then if we introduce noise that makes the labels flip with probability $\eta$ to another class, birds for example, there will be no significant effect on the model's ability to learn the correct class.

Another interesting case is when there is no class confusion and we can assume that $\max_{y} P(y|X) \approx 1$, that is, the clean posterior is almost one-hot. In this case the noisy posterior for a sample $x$ with true class $k$ is given by:
\begin{align}
    \tilde{p}_i &= P(\tilde{y}=i|y, X) \\
    &= \sum_{j} P(\tilde{y}=i|y=j, X)P(y=j|X) \\
    &\approx P(\tilde{y}=i|y=k, X)
\end{align}
which means that the noisy posterior is approximately equal to the transition probabilities of the true class, this is exactly equivalent to the ideal model defined by \cite{northcutt_confident_2021}. In this case, the only necessary condition for a sample to be learnable is that the transition probabilities are maximized for the correct class. That is 
$$P(\tilde{y}=k | y=k, X) > \max_{i \in [1, \dots, \numberofclasses] \backslash k} P(\tilde{y}=i | y=k, X).$$
An interesting conclusion is that when there is no class confusion it is easy to make statements about the global learnability of any problem as long as the transition function does not depend on $x$.

This analysis assumes that no external information is utilized during learning. Incorporating an appropriate regularization method may allow learning the correct label of a sample even if it is not information-theoretic learnable. For instance, if the noise transition function primarily introduces high-frequency label noise---meaning the noise transition function varies much faster than the clean posterior across small regions of the sample space---then applying a regularization method that penalizes high-frequency components in the model's predictions can effectively mitigate this noise.

Moreover, in practice, the observed performance impact when training with label noise may not directly correlate with the concept of learnability. Studies have shown that even when the number of clean samples remain constant, adding samples with symmetric noise can still affect training outcomes even when the noise rate is below the critical point \cite{rolnick_deep_2018}. This suggests that the presence of noisy labels influences model performance beyond the presented learnability concept.

While this concept is not directly applicable in practice, it helps build intuition on how label noise can impact learning. For example, one possible conclusion is that acquiring more data, even with label noise, is a reasonable way to improve results without a specific robust training method. This is supported by the idea that as more data is gathered, it more closely will match the noisy joint distribution. And, for example, in the case of one-hot clean posterior it is extremely unlikely that the noise rate reaches the critical point. This also agrees with the observations made by \cite{rolnick_deep_2018} who demonstrated that deep neural networks achieve high test accuracy even when trained on datasets where clean labels are significantly outnumbered by noisy labels.
